# Supplementary material for: Dr-COVID: Graph Neural Networks for SARS-CoV-2 Drug Repurposing
Source: arXiv:2012.02151 source file (2020-12-03)
Supplement: Supplementary file 1 [file Supporting_info.tex]

\section*{Supporting information}
\paragraph*{S1}
\label{S1}
{\bf COVID-19 predicted drugs using \texttt{Dr-COVID}}. A compiled CSV file of the scores of the drugs predicted using \texttt{Dr-COVID} for the 27 SARS-CoV-2 proteins and 6 coronavirus diseases. 

\paragraph*{S2}
\label{S2}
{\bf COVID-19 predictions using \texttt{GCN}, \texttt{GraphSAGE}, and \texttt{GAT} encoders}. We give three CSV files of the predicted drug scores for the COVID-19 nodes (33 in total) using the three sequential GNN models, namely, \texttt{GCN}, \texttt{GraphSAGE} and \texttt{GAT}.
