# Supplementary material for: Dr-COVID: Graph Neural Networks for SARS-CoV-2 Drug Repurposing
Source: arXiv:2012.02151 source file (2020-12-03)
Supplement: Supplementary file 2 [file appendix.tex]

\section{Appendix} \label{sec:appendix}
    ...
